# Supplementary material for: Using The Concept Hierarchy for Household Action Recognition
Source: arXiv:2409.08853 source file (2024-09-13)
Supplement: Supplementary file 1 [file ch_appendix.tex]

\subsection{Excerpt: Location \textit{ValueDomain}}
A more complex \textit{ValueDomain} than a \textit{Number} is a \textit{Location}, which we have chosen to model as a pair $L = \left(Ref, Pose \right)$, where $Pose$ is the location's pose relative to the reference entity instance $Ref$ or relative to the origin of the environment. We consider that every (household) environment has a fixed, possibly arbitrarily chosen origin, which defines the pose of all physical entity instances inside the environment. For example, if the working environment of a robot is the dining room, the origin of the environment might be at (one of the) the entrance(s) to the room. If a robot manipulator is mounted on a tabletop and its working environment is restricted to just the table, the origin of the environment could be any point on the table, possibly even the mounting point of the manipulator on the table. 

The location of every agent and object instance can be expressed relative to the origin of the environment; however, inspired by \cite{andrei_context_analysis_paper}, we consider it reasonable to represent the location of an instance relative to its \textit{ReferenceObject}. For example, consider the environment in Figure \ref{fig:environment_1}, where the bookshelf is moved to another position. The pose of all the objects inside the bookshelf relative to the bookshelf would not change, contrary to their pose relative to the environment origin. Thus, to save computation time and unnecessary updates, we model the location of instances relative to their \textit{ReferenceObject} and represent the environment instances via a graph.
\begin{figure}[htbp]
    \centering
    \includegraphics[width=1\linewidth]{images/Environment_1_Process_2.png}
    \caption{The workspace of a manipulator robot inside an environment with multiple objects arranged on a bookshelf. Concepts are written in italics, and instances are also underlined.} \label{fig:environment_1}
\end{figure}

To determine an object's \textit{ReferenceObject}, we use a similar procedure as in \cite{andrei_context_analysis_paper}. For that, we defined surfaces of objects and grouped them into surface concepts, such as \textit{ObjectStableSupportSurface}, \textit{SurfaceToSupport}, \textit{PouringSurface}, and others. When constructing the environment location graph, an object, $o_1$, that has a \textit{ObjectStableSupportSurface} in contact with a \textit{SurfaceToSupport} of a different object, $o_2$, is marked as a descendant of $o_2$, which becomes the \textit{ReferenceObject} for $o_1$. Thus, the environment graph in Figure \ref{fig:environment_1_graph} is constructed. If, however, an agent's gripper, e.g., the gripper of a robot or the hand of a person, is in contact with the object, then the \textit{ReferenceObject} of the object is changed to the agent and the location graph is updated accordingly.
\begin{figure}[htbp]
    \centering
    \includegraphics[width=1\linewidth]{images/ConceptHierarchy_Environment1_Graph.png}
    \caption{Part of the location graph of the environment in Figure \ref{fig:environment_1}.} \label{fig:environment_1_graph}
\end{figure}

Because of their relevance in determining the location of objects, we also create the \textit{Gripper} concept inside the hierarchy, with respective subconcepts such as \textit{Hand}, \textit{AntipotalGripper}, \textit{ThreeFingerGripper}, and others, and associate each \textit{AgentInstance} with their corresponding \textit{GripperInstances} according to the embodiment of the agent.

\subsection{Implementation of the Concept Hierarchy} \label{ssec:implementation}
The file containing the concept hierarchy definition is written in JSON format. The hierarchy is split into the concepts and the instances. A parser, written in Python, reads and converts \textbf{only the concepts} inside the JSON file into C++ classes as header and source files that are compiled into a C++ library of concepts. The instances are instantiated with their known properties and values defined in the instances part of the concept hierarchy. All changes to the instances are kept in the program's memory and then updated lazily, after the program finishes, in the concept hierarchy JSON file.

\begin{figure}[!ht]
    \centering
    \includegraphics[width=1\linewidth]{images/ConceptHierarchy_Structure.png}
    \caption{Within a concept hierarchy for household environments, actions, skills, and motion primitives need to be represented, as well as physical entities in the environment, such as objects, surfaces, agents, and grippers. To enable the system to understand the value range of object properties and how they can be modified, \textit{ValueDomains} and \textit{Functions} are modeled. The difference between concepts and instances is explained in \ref{ssec:def_concept_instance}.} \label{fig:concept_hierarchy_first_layer}
\end{figure}

\subsubsection{Syntax}
The syntax of the different subconcept types defined in Figure \ref{fig:concept_hierarchy_first_layer} is individual to reflect the different knowledge modeled in each concept type. The top-concept is defined as in Listing \ref{code:ch_top}. Every concept must define the \texttt{direct_parents} field with its parent concepts and optionally define its specific concept data. The \textit{Concept} root has no data and no parents; it is the root of the hierarchy.
\begin{lstlisting}[language=json,firstnumber=1,caption={Excerpt of the \textit{Object} part of the concept hierarchy showing property definitions and default values.},captionpos=b,label={code:ch_top}]
"Concept": {
  "direct_parents": [],
  "data": {}
},
"PhysicalEntity": {
  "direct_parents": ["Concept"],
  "data": {
    "properties": {
      "instanceName": "String",
      "location": "Location"
    }
  }
},
"Object": {
  "direct_parents": ["PhysicalEntity"],
  "data": {
    "properties": {
      "interactionVolume": "Number",
      "basicShape": "String"
    }
  }
},
"Container": {
  "direct_parents": ["Object"],
  "data": {
    "properties": {
      "content": "Sequence<Object>"
    }
  }
},
"DrinkingMug": {
  "direct_parents": ["Container"],
  "data": {
    "properties": {
      "default": {
        "content": ["Liquid"]
      }
    }
  }
}
\end{lstlisting}

The \textit{PhysicalEntity} concepts define concept properties inside the \texttt{properties} collection as parameter name and its \textit{ValueDomain}. \textit{ValueDomains} are templatable, as ilustrated by the \underline{content} property of the \textit{Container} concept. Default values are specified inside the \texttt{default} property by naming the property and its default value. The specified value must be convertible to the corresponding \textit{ValueDomain}; i.e. serialization and deserialization functions from JSON to each \textit{ValueDomain} must be specified in the code.

\begin{lstlisting}[language=json,firstnumber=2,caption={Instance definition syntax. The mug is located on the ground.},captionpos=b,label={code:instance_def}]
"ObjectInstance": {
  "direct_parents": ["PhysicalEntity"],
  "data": {}
},
"DrinkingMugTUM-MPIInstance": {
  "direct_parents": ["ObjectInstance", 
                     "DrinkingMug"],
  "data": {
    "geometryData": {
      "geometryFile": "../../PerceptionData/data/drinking_mug.json",
      "axis": [0, 0, 1],
      "height": 0.097,
      "radius": 0.0425,
      "displacementFromModelOrigin": [
        [0, 0, 0.0485]
      ],
      "shapeSymmetries": [
        {
          "type": "rotation",
          "axis": [0, 0, 1],
          "axisDisplacementFromOrigin": [0, 0, 0],
          "range": [0, 360]
        }
      ]
    },
    "propertyValues": {
      "interactionVolume": 0.15,
      "basicShape": "cylinder",
      "location": {
        "global": [1.0, 0.0, 0.0, 0.0, 
                   0.0, 0.5, 0.2, 0.0],
        "pose": [1.0, 0.0, 0.0, 0.0, 
                 0.0, 0.5, 0.2, 0.0],
        "rel": "Surface:GroundInstance_
            GroundSupportSurface"
      }
    },
    "surfaces": [
      "DrinkingMugTUM-MPIInstanceBottomSurface", 
      "DrinkingMugTUM-MPIInstanceTopSurface"
    ]
  }
}
\end{lstlisting}

Instance definitions follow a similar structure: in their \texttt{data} field, the \texttt{propertyValues} specify the known property values of the instance, as shown in Listing \ref{code:instance_def}. When the instance is created, unspecified values are filled with the default value of the closest concept or left unknown if no default value is specified for the property. Instances also define their geometry data. The \underline{basicShape} property defines the geometric shape of the object, and the shape's parameters are taken from the \texttt{geometryData} field of the instance's data. If there are defined surfaces of the object, they are entered in the \texttt{surfaces} field of the instance data.

The generated C++ concept classes do not define the properties as member variables. Doing so would make it impossible for a class instance to add, remove, or change one of its concepts during the execution of a program. Thus, we have created a class \textit{ConceptParameters} that has a member variable \underline{properties} of type \texttt{std::map<std::string, std::shared_ptr<ValueDomain>>}. The map's string identifier is the parameter name, and its corresponding value is a specialization of the \textit{ValueDomain} class. We represent UNKNOWN values via a \texttt{nullptr}. The generated C++ concept classes insert in the \textit{ConceptParameters}' \underline{properties} the concept's parameter names and their correct value domain type. A \textit{ConceptParameters} instance does not know the underlying \textit{ValueDomain} of its properties; only the generated concept classes know that.

A physical entity instance is thus represented as a class with a \textit{ConceptParameters} member variable and the list of concepts that the instance is a member of.

The classes for \textit{ValueDomains} are not generated. As explained in \ref{ssec:value_domains}, we let the application designer provide a specialized and optimized implementation of each defined \textit{ValueDomain} in the hierarchy.

Similarly, the implementation of \textit{Functions} is not (necessarily) defined in the concept hierarchy. For defining functions, one needs to specify the \texttt{interface} data by naming and setting the order of \texttt{arguments} and defining the \textit{ValueDomain} of each argument.
\begin{lstlisting}[language=json,firstnumber=3,caption={Functions define interfaces and, optionally, composition schemes.},captionpos=b,label={code:function_def}]
"Function": {
  "direct_parents": ["Concept"],
  "data": {}
},
"Assign": {
  "direct_parents": ["Function"],
  "data": {
    "interface": {
      "arguments": ["who", "what"],
      "who": "ValueDomain",
      "what": "ValueDomain"
    }
  }
},
"Condition": {
  "direct_parents": ["Function"],
  "data": {
    "interface": {
      "arguments": [
        "condition", "ifTrue", "ifFalse"
      ],
      "condition": "Boolean",
      "ifTrue": "Sequence<Function>",
      "ifFalse": "Sequence<Function>"
    }
  }
},
"NumberEquals": {
  "direct_parents": ["Function"],
  "data": {
    "interface": {
      "arguments": ["arg1", "arg2"],
      "arg1": "Number",
      "arg2": "Number",
      "res": "Boolean"
    }
  }
},
"Not": {
  "direct_parents": ["Function"],
  "data": {
    "interface": {
      "arguments": ["arg"],
      "arg": "Boolean",
      "res": "Boolean"
    },
    "procedure": {
      "Condition": {
        "condition": "arg",
        "ifTrue": [
          {
            "Assign": {
              "who": "res",
              "what": false
            }
          }
        ],
        "ifFalse": [
          {
            "Assign": {
              "who": "res",
              "what": true
            }
          }
        ]
      }
    }
  }
},
"NumberNotEquals": {
  "direct_parents": ["Function"],
  "data": {
    "interface": {
      "arguments": ["arg1", "arg2"],
      "arg1": "Number",
      "arg2": "Number",
      "res": "Boolean"
    },
    "procedure": {
      "Assign": {
        "who": "res",
        "what": {
          "Not": {
            "arg": {
              "NumberEquals": {
                "arg1": "arg1",
                "arg2": "arg2"
              }
            }
          }
        }
      }
    }
  }
}
\end{lstlisting}

Optionally, \textit{Functions} can define composition schemes in the \texttt{procedure} field. For composing functions, each argument of the function should be set to a value of its defined \textit{ValueDomain} type. For example, the result of the \textit{NumberNotEquals} function could be computed as $Not(NumberEquals(arg1, arg2)$. In the function definition, the $arg$ parameter of the \textit{Not} function must be set to the result of the \textit{NumberEquals} function, and similarly the $arg1$ and $arg2$ parameters of the \textit{NumberEquals} function must be set to the $arg1$ and $arg2$ parameters of the \textit{NumberNotEquals} function. Thus, function composition can be represented in the Concept Hierarchy.

Definition in JSON; \todo{talk about the definition syntax of skills!}

C++ program; \todo{talk about the graph structure; how we support fast retrieval of isSubConceptOf function checks (maybe analyze the amortized runtime); what the ConceptProperties class represents; the organization of instances: there is only one object instance class but multiple object concept classes; that only define which functions}

\todo{Do we need to provide the code implementation of the details of the concept hierarchy? Do we need to show the meta-learning algorithm in action? Or to show how we implemented the supervision procedure so that no one else is allowed to use the concept hierarchy while it is being restructured and reorganized with the newly added information?}

What performs the post-usage (the meta-learning) phase? This is actually not implemented yet... should we do it also in C++ with a monitoring program that takes charge once the main program is finished (for example, in the destructor of the ConceptHierarchy class)? or make a CRON-Job that periodically calls a bash-script that in turn calls a python script that reorganizes the concept hierarchy and the instances and then regenerates upon change the concept hierarchy classes in C++? One could call the Python script also from C++ by using the \texttt{system} function call...
